# Supplementary material for: KeypointDeformer: Unsupervised 3D Keypoint Discovery for Shape Control
Source: arXiv:2104.11224 source file (2021-04-22)
Supplement: Supplementary file 1 [file control.tex]

\begin{figure*}[h]
  \centering
  \includegraphics[page=1,width=\textwidth]{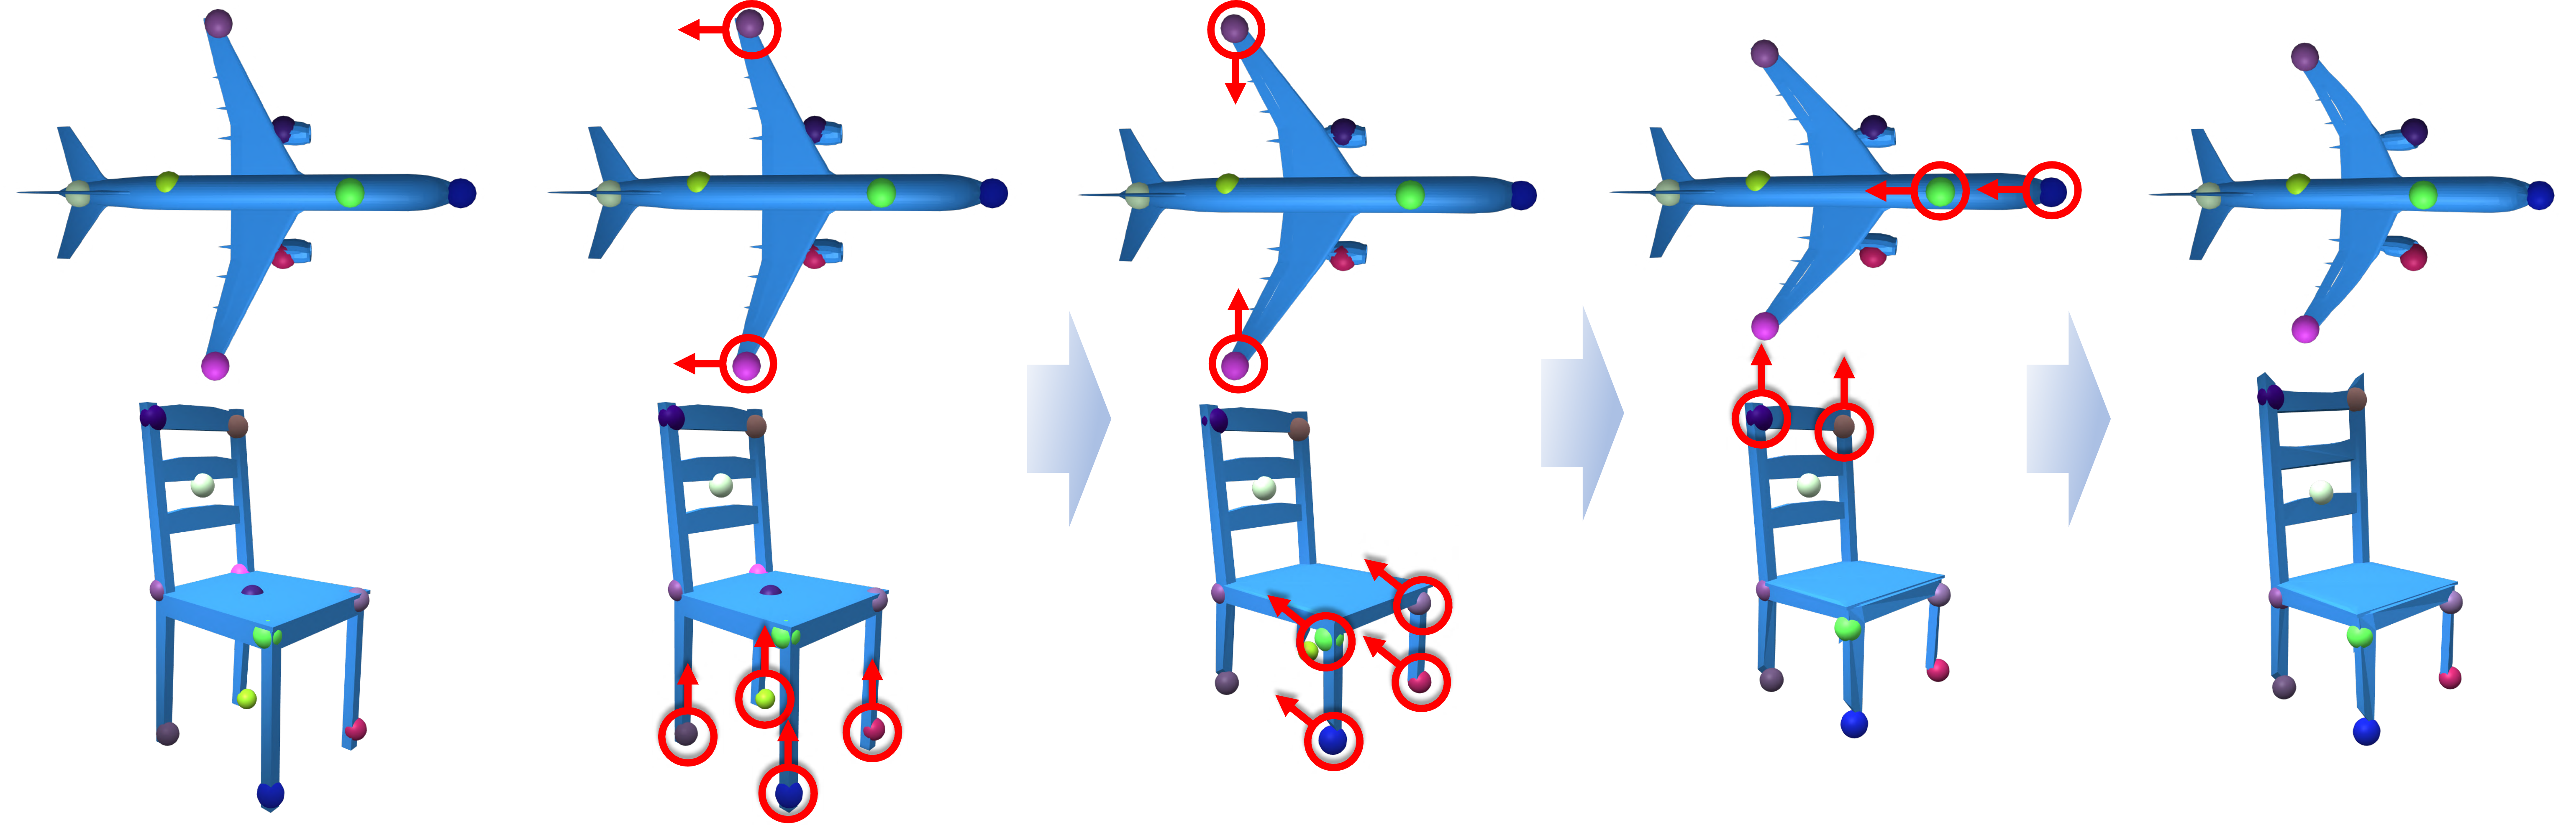}
  \caption{
  \textbf{Shape control via unsupervised 3D keypoints.}
  We show steps from shape editing using our unsupervised 3D keypoints.
  Please refer to our supplementary video on our project page to see the editing in action.
  }\label{sf:control}
\end{figure*}
